# Supplementary material for: Turing patterns on polymerized membranes: a coarse-grained lattice modelling with internal degree of freedom for polymer direction
Source: arXiv:2502.15231 source file (2025-02-21)
Supplement: Supplementary file 1 [file supplementary-material-_1_.pdf]

Cite this: DOI: 00.0000/xxxxxxxxxx

# Turing patterns on polymerized membranes : supplementary material (1)

Fumitake Kato,<sup>a</sup> Hiroshi Koibuchi,<sup>a\*</sup> Elie Bretin,<sup>b</sup> Camille Carvalho,<sup>b</sup> Roland Denis,<sup>b</sup> Simon Masnou,<sup>b</sup> Madoka Nakayama,<sup>c</sup> Sohei Tasaki,<sup>d</sup> and Tetsuya Uchimoto<sup>e,f</sup>

Received Date  
Accepted Date

DOI: 00.0000/xxxxxxxxxx

This supplementary material presents two key elements in the interference between the Turing pattern direction and the mechanical property of the stretched membranes. The first is an order parameter of the internal degree of freedom corresponding to the polymer direction. Secondly, the dependencies of directional energy on the interaction coefficient and the stretching ratio  $R_{xy}$  are discussed.

## 1 Order parameter

First, we calculate the order parameter of the  $x$  component  $\tau^x$  of  $\vec{\tau}$ ;

$$q_\tau^x = 2 \left( \frac{1}{N} \sum_i (\tau_i^x)^2 - 1 \right), \quad (\text{models in } \mathbf{R}^2), \quad (1)$$

$$q_\tau^x = \frac{3}{2} \left( \frac{1}{N} \sum_i (\tau_i^x)^2 - \frac{1}{3} \right), \quad (\text{models in } \mathbf{R}^3).$$

The variable  $\vec{\tau}$  of the models in  $\mathbf{R}^3$  is constrained to be on the tangential plane at vertex  $i$ , and its embedding space is not exactly identified with  $\mathbf{R}^3$ . However, the standard non-polar order parameter, as described in Eq. (1), is employed.

The parameter  $q_\tau^x$  for the models in  $\mathbf{R}^2$  has values in the range  $-1 \leq q_\tau^x \leq 1$ . In the configurations satisfying  $q_\tau^x \simeq 1$  ( $q_\tau^x \simeq -1$ ),  $\vec{\tau}$  is assumed to be parallel to the  $x$ -axis ( $y$ -axis). If the condition  $q_\tau^x \simeq 0$  is satisfied,  $\vec{\tau}$  is assumed to be at random.

The parameter  $q_\tau^x$  for models in  $\mathbf{R}^3$  has values in the range  $-0.5 \leq q_\tau^x \leq 1$ . In the configurations satisfying  $q_\tau^x \simeq 1$  ( $q_\tau^x \simeq -0.5$ ),  $\vec{\tau}$  is assumed to be parallel to the  $x$ -axis (has no component along

the  $x$ -axis). If the condition  $q_\tau^x \simeq 0$  is satisfied,  $\vec{\tau}$  is assumed to be at random. The simulation results are slightly deviated from these criteria, due to the above mentioned fact that the tangential plane is used to define  $\vec{\tau}$ .

### 1.1 Variation of order parameter versus interaction coefficient

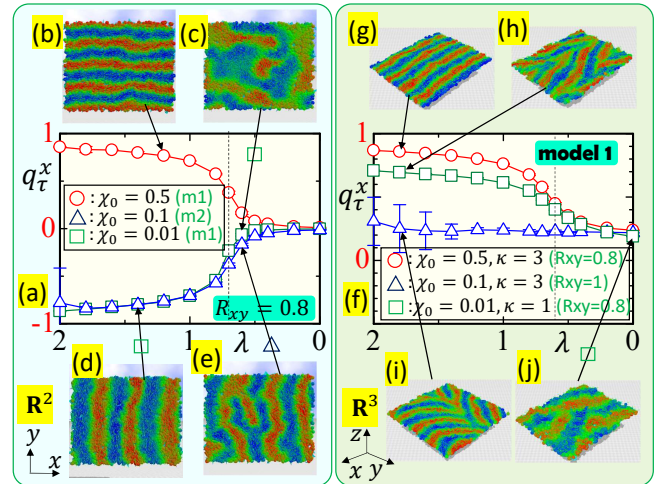

Fig. 1 (a) The order parameter  $q_\tau^x$  vs.  $\lambda$  with (b)–(e) snapshots of the models in  $\mathbf{R}^2$  for  $\chi_0 = 0.5$  ( $\circ$ ),  $\chi_0 = 0.1$  ( $\triangle$ ) and  $\chi_0 = 0.01$  ( $\square$ ), and (f)  $q_\tau^x$  vs.  $\lambda$  with (g)–(j) snapshots of model 1 in  $\mathbf{R}^3$  for three different combinations of the parameters. The dashed vertical line in (a) and (f) represents the position of  $\lambda = 0.6 (\simeq \lambda_c)$ .

As demonstrated in the main text, the parameter  $\lambda$  of the Hamiltonian  $H_\tau$  for the correlation between neighbouring pairs of  $\vec{\tau}$  can be varied in our model. Moreover, the maximum entropy is observed at  $\lambda_c \simeq 0.6$ . It can therefore be concluded that the configurations obtained at  $\lambda = 0.6$  are considered to be representative of those observed in real membranes for all stretching ratios  $R_{xy}$

<sup>a</sup> National Institute of Technology (KOSEN), Ibaraki College, Hitachinaka, Japan, E-mail: katobnbf@ibaraki-ct.ac.jp, koi-hiro@sendai-nct.ac.jp

<sup>b</sup> Institut Camille Jordan (ICJ), CNRS, INSA, Université Claude Bernard Lyon 1, Villeurbanne, France, E-mail: elie.bretin@insa-lyon.fr, camille.carvalho@insa-lyon.fr, denis@math.univ-lyon1.fr, masnou@math.univ-lyon1.fr

<sup>c</sup> Institute for Liberal Arts, Institute of Science Tokyo, Japan, Email: nakayama.madoka@tmd.ac.jp

<sup>d</sup> Department of Mathematics, Hokkaido University, Sapporo, Japan, E-mail: tasaki@math.sci.hokudai.ac.jp

<sup>e</sup> Institute of Fluid Science (IFS), Tohoku University, Sendai, Japan, E-mail: uchimoto@tohoku.ac.jp

<sup>f</sup> ElyTMax, CNRS-Université de Lyon-Tohoku University, Sendai, Japan.

† Electronic Supplementary Information (ESI) available: [details of any supplementary information available should be included here]. See DOI: 10.1039/cXsm00000x/

close to  $R_{xy} = 1$ .

We plot  $q_\tau^x$  vs.  $\lambda$  with the snapshots of TP of the models in  $\mathbf{R}^2$  (Figs. 1(a)–1(e)) and  $\mathbf{R}^3$  (Figs. 1(f)–1(j)). In Fig. 1(a), we find from the data  $q_\tau^x > 0$  ( $\circ$ ) of model 1 (denoted by m1) that the  $\vec{\tau}$  direction is aligned with the  $x$ -axis for  $\chi_0 = 0.5$ . The data  $q_\tau^x < 0$  ( $\triangle$ ) of model 2 indicate that the  $\vec{\tau}$  direction is aligned with the  $y$ -axis. These directions of  $\vec{\tau}$ , as a response to the stretching, are consistent with the TP directions, as shown in the snapshots in Figs. 1(b) and 1(d). In contrast, the data  $q_\tau^x < 0$  ( $\square$ ) of model 1 for  $\chi_0 = 0.01$  are in opposition to the data  $q_\tau^x > 0$  ( $\circ$ ) of model 1 for  $\chi_0 = 0.5$ . The sole distinction between the two data sets is the assumed value of  $\chi_0$ .

Here, we will present the reason why  $\chi_0 = 0.01$  is inadequate for the models that have been assumed. The order parameter  $q_\tau^x$ , which represents the TP direction, at  $\chi_0 = 0.01$  of model 1 in Fig. 1(d) is opposite to that at  $\chi_0 = 0.5$  of model 1 in Fig. 1(b). In the adequate case of Fig. 1(b),  $\Gamma_{ij}^G$  along bond  $ij$  which is almost parallel to the  $x$  axis, is smaller than  $\Gamma_{ij}^G$  along bond  $ij$  which is almost parallel to the  $y$  axis, as discussed in the main text. This results in a larger tensile energy  $H_1$  or bond potential along the  $x$  axis than along the  $y$  axis, which is consistent with the energy transfer under stretching. Similarly, the diffusion energy  $H_u^D$ , represented by the square of the gradient of  $u$ , exhibits a structure analogous to that of the bond potential and thus also undergoes the directional energy transfer (supplementary material (3)). We should recall that the unit Finsler length  $\chi_{ij}$  for  $H_1$  is of the sine type in model 1, whereas it is of the cosine type when applied to  $H_u^D$  irrespective of the models. Consequently, the directional diffusion energy results in a reduction of  $H_u^D$  along the  $x$  axis than along the  $y$  axis, thereby making the TP direction along the  $x$  axis for  $\chi_0 = 0.5$  in model 1.

In contrast, in the inadequate case of Fig. 1(d) for  $\chi_0 = 0.01$ , the value of  $\Gamma_{ij}^G$  along bond  $ij$  that is almost parallel to the  $x$  axis is larger than the value of  $\Gamma_{ij}^G$  along bond  $ij$  that is almost parallel to the  $y$  axis. Therefore, this consequence of the mechanical property by the FG modelling is inconsistent with the configurations stretched along the  $x$  axis: the bond length  $\ell_{ij}$  becomes longer along the  $x$  axis than along the  $y$  axis as a result of the stretching, while the extensive part of the energy  $\ell_{ij}^2$  becomes small in response to the large intensive part  $\Gamma_{ij}^G$ . It is crucial to note that the directional energy transfer in the diffusion energy  $H_u^D$  is not directly controlled by the stretching. Instead, it is indirectly regulated, as the TP direction depends on the  $\vec{\tau}$  direction, which is regulated by the stretching through the FG modelling. Consequently, the TP directions obtained for  $\chi_0 = 0.01$  are also deemed to be non-physical.

The results of  $q_\tau^x$  of model 1 in  $\mathbf{R}^3$  also depend on  $\chi_0$  (Fig. 1(f)). The data ( $\square$ ) for  $\chi_0 = 0.01$  are smaller than those ( $\circ$ ) for  $\chi_0 = 0.5$ . The reason is analogous to the case of the models in  $\mathbf{R}^2$ , where  $\chi_0 = 0.01$  is too small for the purpose of the present study. The large fluctuations in the data ( $\triangle$ ) for large  $\lambda$  region are due to the randomly determined spontaneous TP directions expected under  $R_{xy} = 1$ .

It must be noted that  $q_\tau^x$  ( $\triangle$ ) in Fig. 1(f) for the case of  $R_{xy} = 1$  does not satisfy the condition  $q_\tau^x = 0$ . Instead, it is a positive constant, which implies a violation of the equi-partition theorem that

is universally satisfied in three-dimensional systems. The reason for this violation can be attributed to the fact that, as previously mentioned, the tangential plane at vertex  $i$  is the reference plane for  $\vec{\tau}_i$ , and thus the effective dimension for  $\vec{\tau}_i$  is expected to be smaller than 3.

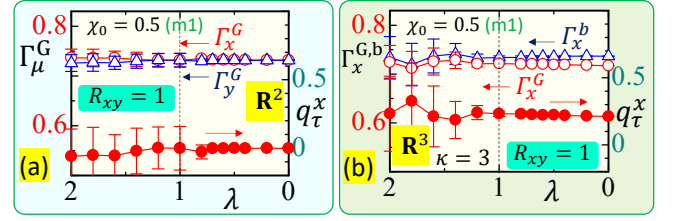

Fig. 2 The order parameter  $q_\tau^x$  ( $\bullet$ ) and coefficients  $\Gamma_{\mu}^{G,b}$  ( $\mu = x, y$ ) ( $\circ, \triangle$ ) of model 1 in (a)  $\mathbf{R}^2$  and (b)  $\mathbf{R}^3$  in the case  $R_{xy} = 1$ .  $\Gamma_x^{G,b}$  are almost the same as  $\Gamma_y^{G,b}$ , which are not depicted in (b). The error bars denote the standard deviation.

It can be deduced that long-range order is not present from the observation that  $q_\tau^x (\simeq 0)$  remains constant. We find from Figs. 2(a),(b) that the models of both  $\mathbf{R}^2$  and  $\mathbf{R}^3$  exhibit this behaviour  $q_\tau^x \simeq 0$  ( $\bullet$ ) in the  $\lambda$  range for  $R_{xy} = 1$  with  $\chi = 0.5$ . Even for large  $\lambda$  regions,  $\vec{\tau}$  aligns along a spontaneous direction only locally, and therefore, no long-range order is expected. For this reason, the corresponding mechanical anisotropy does not appear and the isotropic mechanical property remains unchanged under the  $\lambda$  variation. The  $\Gamma_x^G$  and  $\Gamma_x^b$  plotted in Figs. 2(a),(b) are independent of  $\lambda$ , and the  $y$  components  $\Gamma_y^{G,b}$  (plotted only in Fig. 2(a)) are nearly indistinguishable from  $\Gamma_x^{G,b}$ . This observation indicates an absence of mechanical anisotropy for  $R_{xy} = 1$ .

## 1.2 Variation of order parameter under stretching

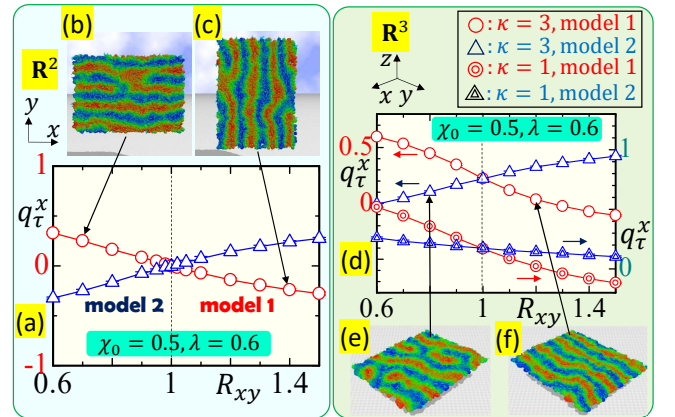

Fig. 3 (a) The order parameter  $q_\tau^x$  vs.  $R_{xy}$  with (b),(c) snapshots of model 1 ( $\circ$ ) and model 2 ( $\triangle$ ) in  $\mathbf{R}^2$  for  $\chi_0 = 0.5$ , and (d)  $q_\tau^x$  vs.  $R_{xy}$  with (e),(f) snapshots of models 1 and 2 in  $\mathbf{R}^3$  for  $\kappa = 3$  and  $\kappa = 1$ . The variation of  $q_\tau^x$  vs.  $R_{xy}$  is compatible with the directional energy transfers, which are presented in the main text.

To confirm the relation between the  $\vec{\tau}$  direction and the energy transfer, we plot  $q_\tau^x$  vs.  $R_{xy}$  with snapshots in Figs. 3(a)–(f) for the models in  $\mathbf{R}^2$  and  $\mathbf{R}^3$ . In Fig. 3(a), the expected behaviour is observed in the variation of  $q_\tau^x$  vs.  $R_{xy}$  of model 1 ( $\circ$ ) and model

2 ( $\triangle$ ) in  $\mathbf{R}^2$  at  $\chi_0 = 0.5$ . This variation of  $q_t^x$  is compatible with the energy transfer from  $H_1^{G,y}$  to  $H_1^{G,x}$  as confirmed in the main text. The data plotted in Fig. 3(d) for the models in  $\mathbf{R}^3$  exhibit an analogous behaviour and are consistent with the energy transfer as observed in the models in  $\mathbf{R}^2$ .

## 2 Variation of directional energy exchange

Here, we discuss the dependencies of the directional energy exchange on the interaction coefficient  $\lambda$  and the stretching ratio  $R_{xy}$ .

### 2.1 Dependence on interaction coefficient and stretching ratio

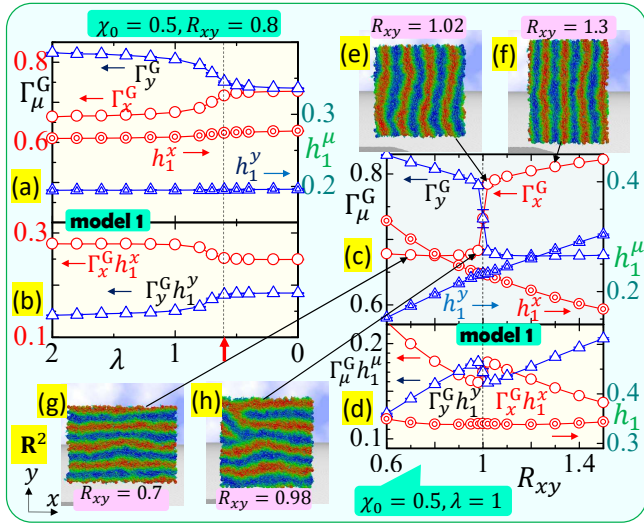

Fig. 4 The directional energy components (a)  $\Gamma_\mu^G$  and  $h_1^\mu$  vs.  $\lambda$ , (b)  $\Gamma_\mu^G h_1^\mu$  vs.  $\lambda$  of model 1 in  $\mathbf{R}^2$  for  $\chi_0 = 0.5$ . (c)  $\Gamma_\mu^G$  and  $h_1^\mu$  vs.  $R_{xy}$  and (d)  $\Gamma_\mu^G h_1^\mu$  and  $h_1$  vs.  $R_{xy}$  with (d)–(h) snapshots of models 1 and 2 in  $\mathbf{R}^2$ . The dashed vertical line on (a) and (b) indicated by  $(\uparrow)$  is the position of  $\lambda = 0.6$ .

The directional components  $\Gamma_\mu^G$  and  $h_1^\mu$  versus  $\lambda$  are plotted in Fig. 4(a), where  $\chi_0 = 0.5$  and  $R_{xy} = 0.8$  are assumed as shown in the figure. We find that  $\Gamma_x^G < \Gamma_y^G$  in the region  $\lambda < \lambda_c (\approx 0.6)$  while the relation  $h_1^x > h_1^y$  remains unchanged. This observation indicates that the condition of (i) in Eq. (58) of Appendix D in the main text is manifest in the range  $\lambda < \lambda_c$ . It is also confirmed that the relation

$$\Gamma_x^G h_1^x > \Gamma_y^G h_1^y \quad (2)$$

remains unchanged under the  $\lambda$  variation (Fig. 4(b)). The simulated data  $\Gamma_\mu^G$  and  $h_1^\mu$  vary abruptly and smoothly, respectively, at  $R_{xy} = 1$  (Fig. 4(c)), and the relations  $\Gamma_x^G h_1^x > \Gamma_y^G h_1^y$  and  $\Gamma_x^G h_1^x < \Gamma_y^G h_1^y$  are exchanged as expected (Fig. 4(d)). This abrupt exchange in the directional energy component at  $R_{xy} = 1$  is reflected in the TP direction, as confirmed by the snapshots in Figs. 4(g)–(f). It should be noted that the data for model 2 are almost identical to those for model 1, except for the TP direction. In the models in  $\mathbf{R}^3$ , the results for sufficiently large  $\kappa$ , such as  $\kappa = 3$ , are almost analogous to those in the models in  $\mathbf{R}^2$ .

It is important to note that the only difference between the conditions for the data presented in this supplementary material (Figs. 4(c)– 4(f)) and those in the main text is the value of  $\lambda$ . In the supplementary material,  $\lambda$  is fixed to  $\lambda = 1$  for the data plotted in Figs. 4(c),(d), while  $\lambda = 0.6$  for the data in Fig. 13(a),(b) in the main text. Since the value of  $\lambda = 0.6$  is associated with the equilibrium configurations of the models, the configurations obtained at  $\lambda = 1$  are considered to be non-equilibrium ones. Consequently, the observed abrupt change in the TP direction with respect to the variation of  $R_{xy}$  is considered to be a potential effect of the non-equilibrium condition, even though the stability condition is satisfied such that  $h_1$  remains unchanged at  $R_{xy}$  close to  $R_{xy} = 1$  (Fig. 4(d)).

## Acknowledgements

This work is supported in part by Collaborative Research Project J24Ly01 of the Institute of Fluid Science (IFS), Tohoku University, and JSPS KAKENHI Grant Number JP23K03225, JP23K03208. Numerical simulations were performed on the supercomputer system AFI-NITY under the project CL01JUN24 of the Advanced Fluid Information Research Center, Institute of Fluid Science, Tohoku University.
