# Supplementary material for: Turing patterns on polymerized membranes: a coarse-grained lattice modelling with internal degree of freedom for polymer direction
Source: arXiv:2502.15231 source file (2025-02-21)
Supplement: Supplementary file 2 [file supplementary-material-_2_.pdf]

Cite this: DOI: 00.0000/xxxxxxxxxx

# Turing patterns on polymerized membranes: supplementary material (2)

Fumitake Kato,<sup>a</sup> Hiroshi Koibuchi,<sup>a\*</sup> Elie Bretin,<sup>b</sup> Camille Carvalho,<sup>b</sup> Roland Denis,<sup>b</sup> Simon Masnou,<sup>b</sup> Madoka Nakayama,<sup>c</sup> Sohei Tasaki,<sup>d</sup> and Tetsuya Uchimoto<sup>e,f</sup>

Received Date  
Accepted Date

DOI: 00.0000/xxxxxxxxxx

In this supplementary material, a detailed exposition of the numerical data on entropy and surface tension is presented. Additionally, the mean value of the coefficient of the Gaussian bond potential is presented.

## 1 Maximum entropy state and related phenomena

The maximum entropy state obtained at  $\lambda = \lambda_c$  is an equilibrium state with the distribution probability  $\exp(-H(\lambda = \lambda_c))$  for any  $R_{xy}$  relatively close to  $R_{xy} = 1$ . It is anticipated that this state will also manifest as an equilibrium state in real membranes. In contrast, a simulated state at  $\lambda \neq \lambda_c$  is not the equilibrium state at  $\lambda = \lambda_c$  because the distribution probability  $\exp(-H(\lambda \neq \lambda_c))$  is different from  $\exp(-H(\lambda = \lambda_c))$ . It can thus be concluded that the simulated state at  $\lambda \neq \lambda_c$  is considered to be a non-equilibrium state in real membranes.

If a membrane for  $R_{xy} = 1$  is immediately stretched to  $R_{xy} = 0.8$ , for instance, then the internal polymer structure will gradually change to the equilibrium structure at  $\lambda = \lambda_c (= 0.6)$ . The relaxation process in the stretched membrane is time-dependent, and therefore, cannot be simulated by the standard MC simulations. Nevertheless, the stretched membrane configuration can be captured within the canonical MC by fixing the initial  $\lambda$  to  $\lambda < 0.6$ .

It is important to note that the ability to describe non-equilibrium states within the canonical modelling framework is a consequence of the incorporation of a novel IDOF, designated as  $\vec{\tau}$ , for the polymer structure. In the extended model, time-dependent phenomena such as relaxation can be described in terms of an equilibrium configuration by controlling  $\vec{\tau}$ . More-

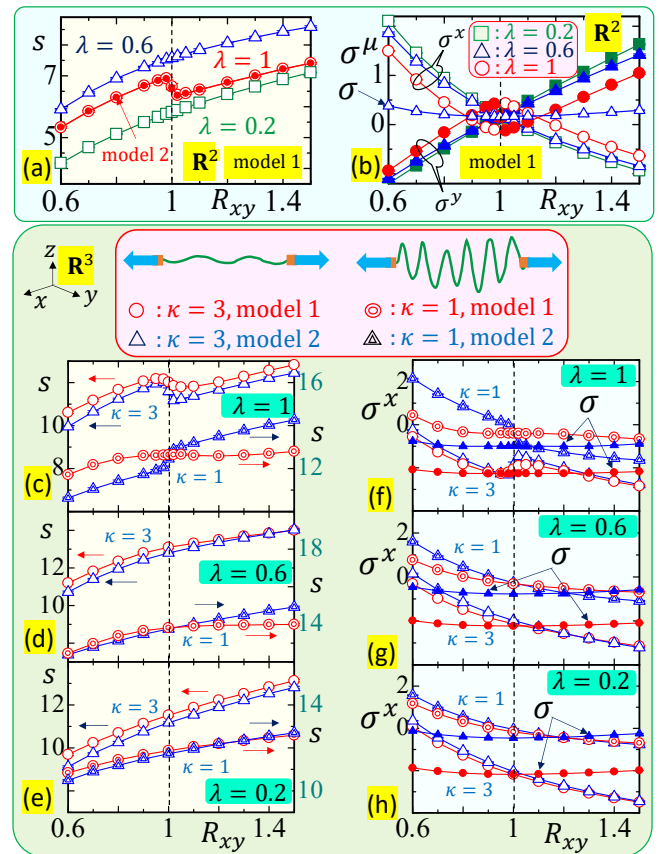

Fig. 1 (a) Entropy  $s(= \delta S / \delta A_p)$  vs.  $R_{xy}$  and (b) surface tension  $\sigma^\mu$ , ( $\mu = x, y$ ) vs.  $R_{xy}$  of model 1 in  $\mathbf{R}^2$  at  $\lambda = 1$  ( $\circ$ ),  $\lambda = 0.6$  ( $\triangle$ ) and  $\lambda = 0.2$  ( $\square$ ). The isotropic  $\sigma$  ( $\triangle$ ) for  $\lambda = 0.6$  is also plotted. The solid symbol ( $\bullet$ ) in (a) represents the results of model 2 at  $\lambda = 1$ . (c)–(h)  $s$  and  $\sigma^x$  of models 1 and 2 in  $\mathbf{R}^3$  for  $\kappa = 1$  and  $\kappa = 3$ . Increasing  $s$ , plotted in (c) represents rubber elasticity. The isotropic  $\sigma$  is also plotted in (f), (g) and (h).

<sup>a</sup> National Institute of Technology (KOSEN), Ibaraki College, Hitachinaka, Japan, E-mail: katobnbf@ibaraki-ct.ac.jp, koi-hiro@sendai-nct.ac.jp

<sup>b</sup> Institut Camille Jordan (ICJ), CNRS, INSA, Université Claude Bernard Lyon 1, Villeurbanne, France, E-mail: elie.bretin@insa-lyon.fr, camille.carvalho@insa-lyon.fr, denis@math.univ-lyon1.fr, masnou@math.univ-lyon1.fr

<sup>c</sup> Institute for Liberal Arts, Institute of Science Tokyo, Japan, Email: nakayama.madoka@tmd.ac.jp

<sup>d</sup> Department of Mathematics, Hokkaido University, Sapporo, Japan, E-mail: tasaki@math.sci.hokudai.ac.jp

<sup>e</sup> Institute of Fluid Science (IFS), Tohoku University, Sendai, Japan, E-mail: uchimoto@tohoku.ac.jp

<sup>f</sup> ELYTMAX, CNRS-Université de Lyon-Tohoku University, Sendai, Japan.

over, the new IDOF enables an accurate representation of energy localisation resulting from the membrane stretching. The energy localisation is linked to time-dependent phenomena in Hamilton's

particle dynamics, as evidenced in the case that the potential energy is dependent on the space variable. Accordingly, an extended model incorporating a new IDOF is indirectly capable of representing time-dependent phenomena, which are non-equilibrium configurations in statistical mechanical viewpoint. The source of this intriguing phenomenon can be attributed to the effective and accurate incorporation of external force-induced interaction anisotropy into the intensive components of energies, namely,  $\Gamma_{ij}^{G,b}(\tau)$  and  $D_{ij}^{u,v}(\tau)$  in Eqs. (5) and (6) in the main text.

Now, we plot  $s$  and the surface tension  $\sigma^\mu$ , ( $\mu = x, y$ ) vs.  $R_{xy}$ , obtained by fixing  $\lambda$  to  $\lambda = 1$ ,  $\lambda = 0.6$  and  $\lambda = 0.2$ , in Figs. 1(a)–(h), where  $\sigma^y$  is plotted only for models in  $\mathbf{R}^2$ . We observe in Fig. 1(a) that  $s$  decrease with decreasing  $R_{xy}$ . This implies that the entropy  $s$  decreases when the surface extends along the  $x$  direction. If we move to the positive direction along the  $R_{xy}$  axis in the region of  $R_{xy} > 1$ , we observe that  $s$  increases. This does not mean the rubber elasticity<sup>1</sup> because the surface is compressed along the  $x$  direction in this case.

As can be seen from Figs. 1(b), it is clear that  $\sigma^x(R_{xy} < 1) > \sigma^x(R_{xy} = 1)$ , which is consistent with the expectation that the surface tension increases with stretching. We find from Fig. 1(b) that  $\sigma^x$  exhibits a gradual increase when  $R_{xy}$  decreases from  $R_{xy} = 1$  for all  $\lambda$ ;  $\lambda = 0.2$  ( $\square$ ),  $\lambda = 0.6$  ( $\triangle$ ) and  $\lambda = 1$  ( $\circ$ ). In the region of  $R_{xy} > 1$ , the surface shape is oblong along the  $y$  direction, where  $\sigma^y$  increases. These responses of  $\sigma^x$  and  $\sigma^y$  to the stretching are physically reasonable.

Results of the models in  $\mathbf{R}^3$  are plotted in Figs. 1(c)–(h), where  $\lambda = 1$ ,  $\lambda = 0.6$  and  $\lambda = 0.2$ . The behaviours of  $s$  and  $\sigma^x$  are nearly analogous to those observed in the models in  $\mathbf{R}^2$ . The entropy is observed to decrease under the stretching.

The isotropic  $\sigma$  ( $\triangle$ ) for  $\lambda = 0.6$  is also plotted in Fig. 1(b). In the case of models in  $\mathbf{R}^2$ ,  $\sigma = 0$  is satisfied when  $(1/N) \sum_{ij} \Gamma_{ij}^G \ell_{ij}^2 \rightarrow 1$  from Eq. (9) in the main text under  $N_{\text{fix}} = 0$ . This condition  $\sigma = 0$  is approximately satisfied when the lattice spacing is given by  $a = 0.525$ , which can be varied depending on the frame area  $A_p (\propto a^2)$  in the case of surfaces with a fixed boundary frame. For the models in  $\mathbf{R}^3$ , the condition for  $\sigma = 0$  is given by  $(1/N) \sum_{ij} \Gamma_{ij}^G \ell_{ij}^2 \rightarrow 3/2$  from Eq. (66) in Appendix E of the main text. However, we assume the same value of  $a = 0.525$  in the simulations for the models in  $\mathbf{R}^3$  independent of  $\kappa$ . For this reason,  $\sigma$  as well as  $\sigma^x$  is negative at  $R_{xy} \rightarrow 1$  for  $\kappa = 3$  in contrast to the case of the models in  $\mathbf{R}^2$ . Nevertheless,  $\sigma$  is close to  $\sigma^x$  at  $R_{xy} \rightarrow 1$  as confirmed from Figs. 1(f)–(h).

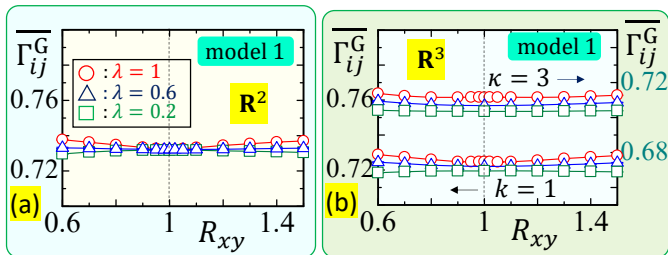

Fig. 2  $\overline{\Gamma_{ij}^G}$  vs.  $R_{xy}$  of model 1 in (a)  $\mathbf{R}^2$  and (b)  $\mathbf{R}^3$  for  $\kappa = 3$  and  $\kappa = 1$ . The parameter  $\lambda$  is fixed to  $\lambda = 1$  ( $\circ$ ),  $\lambda = 0.6$  ( $\triangle$ ) and  $\lambda = 0.2$  ( $\square$ ).

The mean value of  $\overline{\Gamma_{ij}^G} = \frac{1}{N_b} \sum_{ij} \Gamma_{ij}^G$  is plotted in Figs. 2(a),(b)

for model 1 in  $\mathbf{R}^2$  and  $\mathbf{R}^3$ , respectively. Three different values of  $\lambda$  are assumed for both cases of  $\mathbf{R}^2$  and  $\mathbf{R}^3$  as in Fig. 1. We find that  $\overline{\Gamma_{ij}^G}$  is almost independent of the lattice deformation by  $R_{xy}$  in the cases of  $\lambda = 0.6$  ( $\triangle$ ) and  $\lambda = 0.2$  ( $\square$ ). In the case of  $\lambda = 1$  ( $\circ$ ),  $\overline{\Gamma_{ij}^G}$  is slightly influenced by  $R_{xy}$  in the region far from  $R_{xy} = 1$ . It is also noteworthy that the mean values of the coefficients such as  $\Gamma_{ij}^b$  for the models in  $\mathbf{R}^3$  and  $D_{ij}^{u,v}$  are almost independent of  $R_{xy}$ .

## Acknowledgements

This work is supported in part by Collaborative Research Project J24Ly01 of the Institute of Fluid Science (IFS), Tohoku University, and JSPS KAKENHI Grant Number JP23K03225, JP23K03208. Numerical simulations were performed on the supercomputer system AFI-NITY under the project CL01JUN24 of the Advanced Fluid Information Research Center, Institute of Fluid Science, Tohoku University.

## Notes and references

- 1 P. J. Flory, Molecular Theory of Rubber Elasticity, *Polymer Journal*, 1985, 17; No. 1: 1-12, <https://www.nature.com/articles/pj19851.pdf>.
