# Supplementary material for: Turing patterns on polymerized membranes: a coarse-grained lattice modelling with internal degree of freedom for polymer direction
Source: arXiv:2502.15231 source file (2025-02-21)
Supplement: Supplementary file 3 [file supplementary-material-_3_.pdf]

Cite this: DOI: 00.0000/xxxxxxxxxx

# Turing patterns on polymerized membranes: supplementary material (3)

Fumitake Kato,<sup>a</sup> Hiroshi Koibuchi,<sup>a\*</sup> Elie Bretin,<sup>b</sup> Camille Carvalho,<sup>b</sup> Roland Denis,<sup>b</sup> Simon Masnou,<sup>b</sup> Madoka Nakayama,<sup>c</sup> Sohei Tasaki,<sup>d</sup> and Tetsuya Uchimoto<sup>e,f</sup>

Received Date  
Accepted Date

DOI: 00.0000/xxxxxxxxxx

The focal point of this supplementary material is the diffusion energy localization of the chemical reactants  $u$  and  $v$ . Additionally, the relationship between the diffusion direction of  $u$  and  $v$  and the polymer direction is also explored.

## 1 Diffusion energy localisation

The directional TP system  $(u, v)$  is also expected to appear on the stretched membranes in both models such that the TP direction is identical with the direction along which the diffusion energy is smaller. To illustrate how the diffusion energy transfers are observed, we plot the direction-dependent diffusion coefficients  $D_{\mu}^{u,v}$ , ( $\mu = x, y$ ) and energies  $D_{\mu}^{u,v} h_{u,v}^{D,\mu} (= D_{\mu}^{u,v} H_{u,v}^{D,\mu} / N_B)$ , ( $\mu = x, y$ ) of model 1 in Figs. 1(a)–(g), where  $\kappa = 3$ .

The snapshots are normalized diffusion energies  $h_u^D (= H_u^D / N_B)$  and  $h_v^D (= H_v^D / N_B)$  corresponding to those of TPs in Fig. 14 in the main text. The total number of lines is twice as large as the number of TPs, as the values of  $h_u^D$  and  $h_v^D$  are defined by the squares of first-order differentials, which are identical at the increasing and decreasing parts of  $u$  and  $v$  along the TPs.

As a consequence of the stretching of the membranes, the diffusion energies of  $u$  and  $v$  are divided into two parts such that

$$H_u^D = D_x^u H_u^{D,x} + D_y^u H_u^{D,y}, \quad H_v^D = D_x^v H_v^{D,x} + D_y^v H_v^{D,y}, \quad (1)$$

where the  $z$  components are ignored. In the expressions, the  $D_{\mu}^{u,v}$ , ( $\mu = x, y$ ) satisfy  $D_x^{u,v} = D_y^{u,v}$  in the case of the unstretched membranes ( $\Leftrightarrow R_{xy} = 1$ ). In contrast, the results  $D_x^{u,v} \neq D_y^{u,v}$  are caused by the  $\vec{\tau}$  orientation on the stretched membranes ( $\Leftrightarrow R_{xy} \neq 1$ ).

The energy data in Figs. 1(b),(c) show how the isotropic dif-

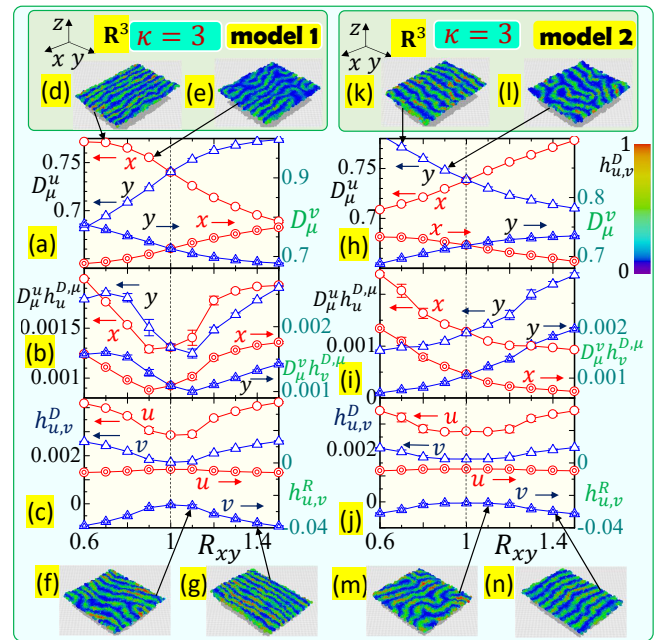

Fig. 1 Direction-dependent diffusion coefficient  $D_{\mu}^{u,v}$ , the direction-dependent diffusion energies  $D_{\mu}^{u,v} h_{u,v}^{D,\mu} (= D_{\mu}^{u,v} H_{u,v}^{D,\mu} / N_B)$  and  $h_{u,v}^{D,\mu} (= H_{u,v}^{D,\mu} / N_B)$  with snapshots of (a)–(g) model 1 and (h)–(n) model 2 for membranes in  $\mathbf{R}^3$  for  $\kappa = 3$ , where  $R_{x,y} = 0.8$ . The snapshots are normalized diffusion  $h_u^D$  energies in (d),(e),(k),(l) and  $h_v^D$  in (f),(g),(m),(n).

<sup>a</sup> National Institute of Technology (KOSEN), Ibaraki College, Hitachinaka, Japan, E-mail: katobnbj@ibaraki-ct.ac.jp, koi-hiro@sendai-nct.ac.jp

<sup>b</sup> Institut Camille Jordan (ICJ), CNRS, INSA, Université Claude Bernard Lyon 1, Villeurbanne, France, E-mail: elie.bretin@insa-lyon.fr; camille.carvalho@insa-lyon.fr; denis@math.univ-lyon1.fr; masnou@math.univ-lyon1.fr

<sup>c</sup> Institute for Liberal Arts, Institute of Science Tokyo, Japan, Email: nakayama.madoka@tmd.ac.jp

<sup>d</sup> Department of Mathematics, Hokkaido University, Sapporo, Japan, E-mail: tasaki@math.sci.hokudai.ac.jp

<sup>e</sup> Institute of Fluid Science (IFS), Tohoku University, Sendai, Japan, E-mail: uchimoto@tohoku.ac.jp

<sup>f</sup> ElyTMax, CNRS-Université de Lyon-Tohoku University, Sendai, Japan.

fusion systems are activated to the directional TP system  $(u, v)$  by the interactions  $f, g$  and by the stretching. The plots of  $h_{u,v}^{D,R}$  in Figs. 1(c),(j) indicate that  $H_{u,v}^D$  and  $H_{u,v}^R$  in Eqs. (50) and (51) in the main text are positively and negatively increasing, respectively, under the stretching. The result  $h_u^D > h_v^D$  at  $R_{xy} = 1$  in Fig. 1(c) indicates the occurrence of non-trivial and non-directional energy transfer, due to the interactions  $f$  and  $g$ , between the diffusion systems of  $u$  and  $v$ . These diffusion systems are initially spatially uniform with zero diffusion energy in the absence of interactions. Note that the TP system  $(u, v)$  at  $R_{xy} = 1$  corresponds

to non-equilibrium steady state resulting from the non-trivial interactions  $f$  and  $g$  in Eq. (2) in the main text.

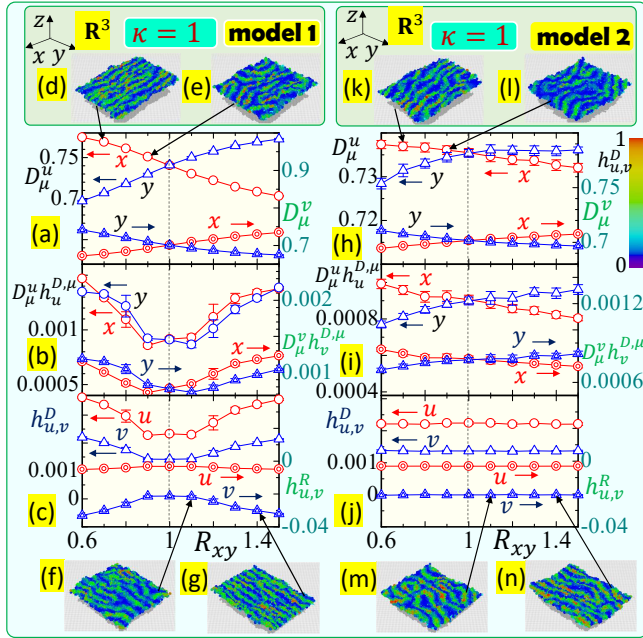

Fig. 2 Direction-dependent diffusion coefficient  $D_{\mu}^{u,v}$ , the direction-dependent diffusion energies  $D_{\mu}^{u,v} h_{u,v}^{D,\mu} (= D_{\mu}^{u,v} H_{u,v}^{D,\mu} / N_B)$ , and  $h_{u,v}^{D,R} (= H_{u,v}^{D,R} / N_B)$  with snapshots of (a)–(g) model 1 and (h)–(n) model 2 for membranes in  $R^3$  for  $\kappa=1$ , where  $R_{xy}=0.8$ . The snapshots are normalized diffusion energies  $h_u^D$  in (d),(e),(k),(l) and  $h_v^D$  in (f),(g),(m),(n).

The results of model 2 are plotted in Figs. 1(h)–(n), where  $D_{\mu}^{u,v} h_{u,v}^{D,\mu}$ , ( $\mu=x,y$ ) in Fig. 1(i) are almost symmetric to those of model 1 in Fig. 1(b) under the exchange  $x \leftrightarrow y$  as expected from the difference in  $\chi_{ij}^u$  and  $\chi_{ij}^v$  in Eqs. (7), (8) in the main text. The directional diffusion energy transfer is apparent only in model 2. However, the observed relations between  $D_{\mu}^{u,v} h_{u,v}^{D,\mu}$ , ( $\mu=x,y$ ) are consistent with the TP direction expected to appear in the smaller  $D_{\mu}^{u,v} h_{u,v}^{D,\mu}$  in both models.

The results obtained for  $\kappa=1$  are presented in Figs. 2(a)–(n). The data for model 1 in Figs. 2(a)–(g) are almost the same as those for  $\kappa=3$  in Figs. 1(a)–(g). The data of model 2 plotted in Figs. 2(h),(i) are different from those of model 1 in Figs. 1(h),(i). The behaviours of  $h_{u,v}^{D,\mu}$  vs.  $R_{xy}$  are the same as those of  $D_{\mu}^{u,v} h_{u,v}^{D,\mu}$ , and therefore, the data in Figs. 1(h),(i) and Figs. 2(h),(i) satisfy one of the conditions

$$\begin{aligned} D_x^u < D_y^u &\Leftrightarrow H_u^{D,x} > H_u^{D,y}, \\ D_x^v < D_y^v &\Leftrightarrow H_v^{D,x} > H_v^{D,y}, \end{aligned} \quad (2)$$

and

$$\begin{aligned} D_x^u > D_y^u &\Leftrightarrow H_u^{D,x} > H_u^{D,y}, \\ D_x^v > D_y^v &\Leftrightarrow H_v^{D,x} > H_v^{D,y}, \end{aligned} \quad (3)$$

where  $>$  and  $<$  can be exchanged in both sides of " $\Leftrightarrow$ ". These correspond to Eqs. (30) and (31) in the main text for the membrane energy localisation. The TP directions of  $h_u^D$  and  $h_v^D$  appear

in the direction along the lower diffusion energies  $H_u^{D,\mu}$  and  $H_v^{D,\mu}$  for  $\kappa=3$ , however, these relations are reversed for  $\kappa=1$  in model 2.

It is important to provide commentary on the relationship between the TP direction and the directional diffusion of chemical reactants  $u$  and  $v$ . As described above, the diffusion direction of  $u$  and  $v$  are identical with the TP directions, which is analogous to the polymer direction  $\vec{\tau}$ . This analogy is exemplified by the snapshots presented in the main text. Consequently, the diffusion direction of  $u$  and  $v$  is found to be parallel to the polymer direction in both model 1 and model 2 on the stretched polymerized membranes.

## Acknowledgements

This work is supported in part by Collaborative Research Project J24Ly01 of the Institute of Fluid Science (IFS), Tohoku University, and JSPS KAKENHI Grant Number JP23K03225, JP23K03208. Numerical simulations were performed on the supercomputer system AFI-NITY under the project CL01JUN24 of the Advanced Fluid Information Research Center, Institute of Fluid Science, Tohoku University.
